# Supplementary material for: Research Challenges in Orchestration Synthesis
Source: arXiv:2308.10651 source file (2023-08-23)
Supplement: Supplementary file 1 [file appendix.tex]

\newpage
\section{Appendix}

\begin{definition}[Refined Semi-Controllability]\label{def:refinedsemicontrollability}
Let $\mathcal A$ be an MSCA and let $t = (\vec q_t, \vec a_t, \vec q_t\!') \in T^{\Box_l}_{\mathcal A}$. 
Moreover, given $\mathcal A'\subseteq\mathcal A$, if  
$\exists\,t' = (\vec{q_{t'}}, \vec {a_{t'}}, \vec{q_{t'}}\!') \in T^{\Box_l}_{{\mathcal A}'}$ in $\mathcal A'$ such that the following hold:
\begin{enumerate}
    \item\label{semi:1} 
$\vec a_{t'}$ is a match,  
$\vec q_{t'}, \vec q_{t'}\!' \not\in \textit{Dangling\/}(\mathcal A')$,
$\ithel{\vec{q}_{t}{}}{j} = \ithel{\vec{q}_{t'}{}}{j}$,  $\ithel{\vec{a}_{t}{}}{j} = \ithel{\vec{a}_{t'}{}}{j} = ?a$, for some $j \in 0 \ldots rank(\mathcal A)$;
and 
\item\label{semi:2} there exists a sequence of 
 transitions 
 $t_0, \ldots, t_n$ of $\mathcal A'$ such that 
 $\forall i \in 0\ldots n$,  
$t_i=(\vec{q_i},\vec{a_i},\vec{q_i}')$ and the following hold:
\begin{itemize}
 \item $\vec q_0=\vec q_{t}$; 
 \item $t_n = t'$;
 \item 
$\vec{q_i},\vec{q_i}' \not \in Dangling(\mathcal A ')$; and
\item if $i<n$, then $\ithel{\vec{a_i}}{j}=-$ and  $\vec{q_i}'=\vec{q}_{i+1}$;
\end{itemize}
\end{enumerate}
then $t$ is \emph{controllable\/} in $\mathcal A'$ (via $t'$).
Otherwise, $t$ is \emph{uncontrollable\/} in $\mathcal A'$.
\end{definition}

%%%%%%%%%%%%%%%%%%%%%%%%%%%%%%%%%%%

\begin{definition}[??? Semi-Controllability]\label{def:?semicontrollability}
Let $\mathcal A$ be an MSCA and let $t = (\vec q_t, \vec a_t, \vec q_t\!') \in T^{\Box_l}_{\mathcal A}$, where the principal at index $j$ performs the necessary request, formally   
 $\ithel{\vec{a}_{t}{}}{j}\!\in \Rset\ $ for some $j \in 0 \ldots rank(\mathcal A)$, where  
 $\Pi^j(\mathcal A)= \mathcal A_j$ is the $j$-th principal.  
Moreover, given $\mathcal A'\subseteq\mathcal A$, 
if  there exists $\vec q \in Q_{\mathcal A'} \not \in  \textit{Dangling\/}(\mathcal A')$ such that  for all $?a \in \Rset$ such that $\ithel{\vec{q}_{t}{}}{j} \TRANSS{[?a]_{\Box_l}}   \in T_{\mathcal A_j}$, 
 there exists $t' = (\vec{q_{t'}}, \vec {a_{t'}}, \vec{q_{t'}}\!') \in T^{\Box_l}_{{\mathcal A}'}$ in $\mathcal A'$ such that the following hold:
\begin{enumerate}
    \item\label{semi:1} 
$\vec a_{t'}$ is a match,  
$\vec q_{t'}, \vec q_{t'}\!' \not\in \textit{Dangling\/}(\mathcal A')$,
$\ithel{\vec{q}_{t}{}}{j} = \ithel{\vec{q}_{t'}{}}{j}$, 
$\ithel{\vec{a}_{t'}{}}{j} = ?a$, 
and 

\item  there exists a sequence of 
 transitions 
 $t_0, \ldots, t_n$ of $\mathcal A'$ such that 
 $\forall i \in 0\ldots n$,  
$t_i=(\vec{q_i},\vec{a_i},\vec{q_i}')$ and the following hold:
\begin{itemize}
 \item $\vec q_0=\vec q$; 
 \item $t_n = t'$;
 \item 
$\vec{q_i},\vec{q_i}' \not \in Dangling(\mathcal A ')$; and
\item if $i<n$, then $\ithel{\vec{a_i}}{j}=-$ and  $\vec{q_i}'=\vec{q}_{i+1}$;
\end{itemize}
\end{enumerate}
\noindent
then $t$ is \emph{controllable\/} in $\mathcal A'$ (via $\vec q$).
Otherwise, $t$ is \emph{uncontrollable\/} in $\mathcal A'$.
\end{definition}

This definition is wrong as it computes the orchestration of the first example, which should be empty. 
I would like to show that if there is no orchestration with Def.~\ref{def:?semicontrollability} then there is no orchestration with Def.~\ref{def:refinedsemicontrollability}. 
Apparently, Def.~\ref{def:refinedsemicontrollability} appears to be a special case of Def.~\ref{def:?semicontrollability}. 
This means that it seems that Def.~\ref{def:?semicontrollability} renders more transitions uncontrollable then 
Def.~\ref{def:refinedsemicontrollability}. 
This is counter-intuitive as apparently, it implies the converse, i.e., if there is no orchestration with Def.~\ref{def:refinedsemicontrollability} then there is no orchestration with Def.~\ref{def:?semicontrollability}.  
We know that this is not true by Example~\ref{ex:card}. 
The reason is that to render a state bad it suffices to have one outgoing uncontrollable bad transition, hence 
it does not matter if the other outgoing transitions are uncontrollable or not.
